# Supplementary material for: Compositional Chain-of-Thought Prompting for Large Multimodal Models
Source: arXiv:2311.17076 source file (2024-04-01)
Supplement: Supplementary file 2 [file archived_tbl_4_supp.tex]

% \definecolor{mediumgray}{gray}{0.8}
%Note to anyone using this template in the future ? will give you bold vertical lines, while | is regular
% % Adjust row height
\renewcommand{\arraystretch}{1.1}
\newcolumntype{?}{!{\vrule width 2 pt}}
\newcolumntype{P}[1]{>{\centering\arraybackslash}p{#1}}
\newcolumntype{G}[1]{>{\columncolor{lightgray}\centering\arraybackslash}p{#1}}
% \begin{center}
\begin{table*}[t]
\begin{center}
\begin{tabular}{m{0.18\textwidth}G{0.08\textwidth}G{0.08\textwidth}G{0.08\textwidth}P{0.08\textwidth}P{0.08\textwidth}P{0.08\textwidth}P{0.08\textwidth}}%P{0.08\textwidth}}
        \multicolumn{1}{c}{}& \multicolumn{3}{c}{\textbf{Multimodal Benchmarks}} & \multicolumn{4}{c}{\textbf{VL Compositional Benchmarks}} \\
        \toprule
        Model & SEED-I & MMB & LLaVA-Bench & Wino-Text & Wino-Image &Wino-Group & WHOOPS! VQA BEM   \\ \hline
        CLIP & - &  - & - & 30.7 & 10.5 & 8.0 & -  \\
        BLIP & - &  - & - & 39.0 & 19.2 &  15.0 & 39.0  \\
        BLIP2 & 46.4 & - & - & 42.0 & 23.8 & 19.0 & 55.0 \\
        SGVL$^\dag$ & - &  - & - & {42.8}\dag & {28.5}\dag & {23.3}\dag & - \\
        mPlug-OWL2 & 57.8 &  64.5 & - & - & - & - & -  \\
        QwenVL-Chat & 58.2 &  61.2 & - & - & - & - & - \\ \hline
        InstructBLIP & 48.2 &  36.0 & 47.7 & 7.0 & 11.5& 3.3  & 48.7  \\ 
        InstructBLIP-ZS-CoT & 37.6 & 25.3 & 42.0 & 9.3 & 16.3 & 4.0 & 30.8 \\
        \textbf{InstructBLIP-{\smodel}} & 56.9\gcol{+8.7} &40.3\gcol{+4.3}& 48.1 \gcol{+0.4} &21.0\gcol{+14.0} & 21.3\gcol{+9.8} & 8.3\gcol{+5.0} & \textbf{59.9}\gcol{+11.2}\\ \hline
        %InternLM-XC & 60.5 &  74.4& 18.0 & 23.0 & 8.5 & 62.6 & - \\
        %InternLM-XC-ZS-CoT &58.9 & ? &19.7& 20.7 & 10.0 & 61.6 & - \\
        %\textbf{InternLM-XC-{\smodel}} & ? & ?&17.5\rcol{-0.5} & 27.0\gcol{+4.0} & 8.0\rcol{-0.5} & ? & - \\ \hline
        LLaVA-1.5 & 68.4 &  67.0 & 70.1 & 36.0 & 33.3 & 20.1 & 47.9 \\
        LLaVA-1.5-ZS-CoT & 66.7 &66.0 & 61.0 &28.0& 22.5&12.3&46.0  \\
        \textbf{LLaVA-1.5-{\smodel}} & \textbf{69.9}\gcol{+1.5} & \textbf{70.7}\gcol{+3.7} & \textbf{70.4} \gcol{+0.3} &\textbf{42.0}\gcol{+6.0} & \textbf{35.5}\gcol{+2.2}&\textbf{22.3}\gcol{+2.2} & 48.9\gcol{+1.0} \\ \bottomrule
    \end{tabular}
    \end{center}
% \vspace{-3mm}
\caption{\textbf{Main results table with additional benchmarks} Abbreviations: SEEDBench-Image [SEED-I]; MMBench [MMB]; Winoground Text Score: Wino-Text, Image Score: Wino-Image, Group Score: Wino-Group. Unlike our zero-shot approach, models with \dag\ are supervised and finetuned on annotated scene graphs. }
\label{tbl: main_supp}
\end{table*}
% \end{center}
